# Supplementary material for: Modelling to Generate Continuous Alternatives: Enabling Real-Time Feasible Portfolio Generation in Convex Planning Models
Source: arXiv:2411.16887 source file (2024-11-25)
Supplement: Supplementary file 1 [file SI.tex]

\paragraph{} MOO thoroughly explores the trade-offs between the set of objectives put into the model by the modelling team. Because it requires the set of pertinent objectives to be known before hand, MOO is ideal for situations where a limited number of predecided objectives need to be explored to answer a given research question. For instance, academic studies focused on a few metrics of interest or reports with for a known set of stakeholders with a feedback mechanism that allows those stakeholders to communicate their priorities and have them reflected in model formation. In these settings, MOO is able to represent all important objectives and communicate the trade-off space in pertinent metrics created by the set of Pareto optimal decisions. There are, however, a number of challenges associated with MOO in a decision support context. First, it does not typically save any Pareto inefficient solutions. While the Pareto efficient solutions do form the set of best possible outcomes, they show no inefficient outcomes in the selected metrics, whether that takes the form of Pareto optimal solutions to an objective that was not included or simply non-optimal choices, which may result from human inefficiency or from an unforeseen constraint like opposition to transmission siting.  Thus, the Pareto set will consistently underestimate the full set of potential solutions within budget, even if it does heavily sample the optimal trade-off space. Second, as mentioned before, MOO also requires the foreknowledge of all objectives of interest to all stakeholders involved. While this is possible for some very targeted reports, or reports with vast survey work carried out ahead of time, in many studies the important objective statements will be assumed by the researchers, adding an additional source of uncertainty. Importantly, the addition of new objective statements specified by stakeholders requires rerunning the model multiple times, inducing significant usage of computational time and resources, and a substantial time lag for the stakeholder. These characteristics make MOO difficult to apply in a live, decision support system usable by many stakeholders.

Please note that the following methods can be used individually or in conjunction with one another.
